# Supplementary material for: Learning to Control Emulated Muscles in Real Robots: Towards Exploiting Bio-Inspired Actuator Morphology
Source: arXiv:2402.05371 source file (2024-02-08)
Supplement: Supplementary file 1 [file suppl_content.tex]

\appendix

\subsection{Simulation Engines}
\label{supp:sim}
